# Supplementary material for: Doping Dependence of Collective Spin and Orbital Excitations in Spin 1 Quantum Antiferromagnet La$_{2-x}$Sr$_x$NiO$_4$ Observed by X-rays
Source: arXiv:1612.06903 ancillary file (2017-02-17)
Supplement: Supplementary file 1 [file Supplemental_Material.pdf]

# Supplemental Material for: Doping Dependence of Collective Spin and Orbital Excitations in Spin 1 Quantum Antiferromagnet $\text{La}_{2-x}\text{Sr}_x\text{NiO}_4$ Observed by X-rays

G. Fabbri\*, D. Meyers, L. Xu, V. M. Katukuri, L. Hozoi, X. Liu, Z.-Y. Chen, J. Okamoto, T. Schmitt, A. Uldry, B. Delley, G. D. Gu, D. Prabhakaran, A. T. Boothroyd, J. van den Brink, D. J. Huang, and M. P. M. Dean<sup>†</sup>  
(Dated: February 16, 2017)

This document provides further details and supporting measurements for the main manuscript. The experimental geometry for the resonant inelastic x-ray scattering (RIXS) measurements is depicted in Fig. S1. Fits of  $\text{La}_2\text{NiO}_4$  RIXS lineshape are shown in Fig. S2. Further details on the RIXS simulations used in this work are provided together with calculations for a mixture of atomic Ni  $3d^7$  and  $3d^8$  that we show to be inconsistent with the experimental results for  $\text{La}_{1.66}\text{Sr}_{0.33}\text{NiO}_4$ . The large dichroism observed in the  $\text{La}_2\text{NiO}_4$  RIXS is displayed in Fig. S4. Finally, linecuts of the doping dependence of the LSNO RIXS are presented as further evidence of the much larger reconstruction of its charge and orbital excitations when compared to cuprates.

## SCATTERING GEOMETRY

The experimental geometry is displayed in Fig. S1. Linearly polarized x-rays are incident at  $\theta_i$  on the sample, which has a  $c$ -axis surface normal. Most measurements shown in the manuscript were performed with horizontally polarized x-rays ( $\pi$ ), except for the RIXS temperature dependence displayed in Fig. 4(c) of the main

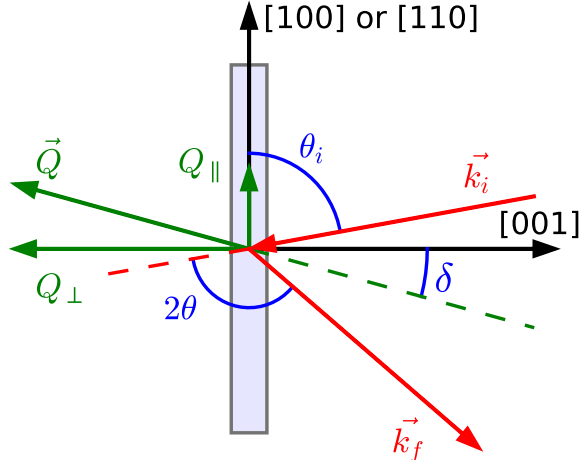

FIG. S1. RIXS scattering geometry. Linearly polarized x-rays with wavevector  $\vec{k}_i$  are incident upon the sample. The scattered photons ( $\vec{k}_f$ ) are collected at  $2\theta = 130^\circ$  and measured as a function of final energy, thus the magnitude of the in-plane transferred moment ( $Q_{\parallel}$ ) is controlled by  $\delta$ .

manuscript. The magnetic excitations of  $\text{La}_{2-x}\text{Sr}_x\text{NiO}_4$  are highly two dimensional [1], thus the magnon dispersion is a function of  $Q_{\parallel}$ . In this geometry, the amplitude of  $Q_{\parallel}$  is determined by

$$Q_{\parallel} = 2|k_i| \sin(2\theta/2) \sin(\delta), \quad (1)$$

where  $|k_i| = 0.433 \text{ \AA}^{-1}$  for the Ni  $L_3$ -edge,  $2\theta$  is fixed at  $130^\circ$ , and we vary  $Q_{\parallel}$  by changing  $\delta$ . The magnetic dispersion is measured along  $[\pi, 0]$  and  $[\pi, \pi]$  by rotating the sample around the  $[001]$  axis.

## FITS OF THE RIXS LINESHAPE

The lineshape of the magnetic excitations observed in the RIXS spectra of  $\text{La}_2\text{NiO}_4$  is best adjusted using a model with three pseudo-Voigt functions (Fig. S2). The energy calibration and resolution function were obtained from measurements of a carbon tape immediately before and after each sample scan. Since the peaks observed in  $\text{La}_{2-x}\text{Sr}_x\text{NiO}_4$  (LSNO) largely overlap, we applied the following constraints in order to reduce the number of independent variables: the elastic line was fixed at zero energy, the width of all three peaks were fixed to that measured in the carbon tape, and the multi-magnon excitation peak was fixed to double of the magnon bandwidth (252 meV for  $x = 0$ ). Note that the small dispersion of multi-magnons is not only suggested by theory [2] but seen in the raw data at low  $Q_{\parallel}$  [see for instance  $Q_{\parallel} = (0.06\pi, 0.06\pi)$  in Fig. S2].

## CALCULATIONS DETAILS

We used *ab initio* quantum chemistry calculations to simulate the Ni  $3d$  orbital and magnetic excitations observed by RIXS. Furthermore, crystal field parameters were extracted by optimizing the agreement with the experimental data and atomic calculations. These methods are detailed below.

### *Ab initio* quantum chemistry calculations

#### Ni $3d$ -shell excitations

To analyse the Ni  $3d^8$  multiplet structure, we have performed many-body calculations using wavefunc-

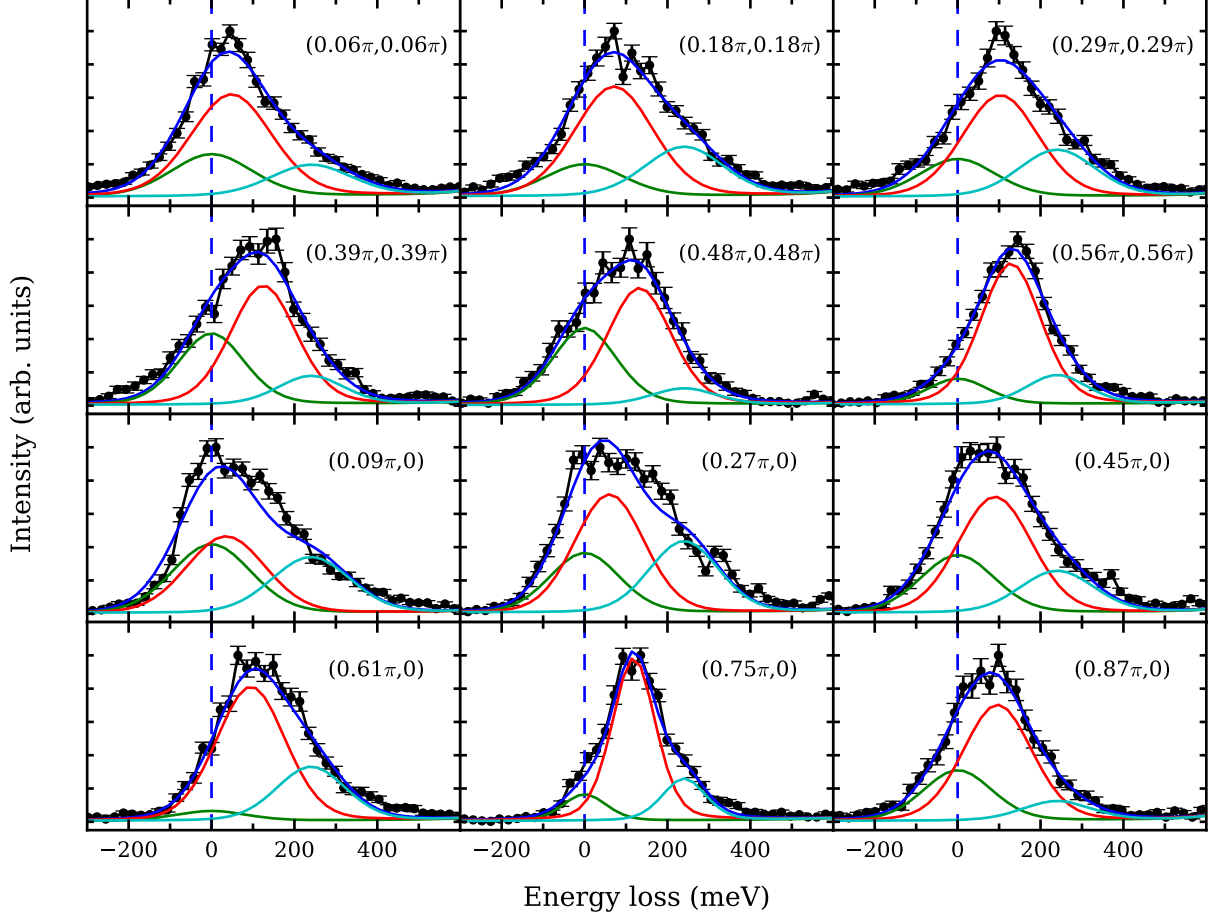

FIG. S2. Fits of the  $\text{La}_2\text{NiO}_4$  Ni  $L_3$  edge RIXS  $Q_{\parallel}$  dependence.

tion quantum chemistry methods. The calculations were based on complete-active-space self-consistent-field (CASSCF) and multireference configuration-interaction (MRCI) techniques [3]. An embedded cluster consisting of a central  $\text{NiO}_6$  octahedron, 4 nearest-neighbor (NN)  $\text{NiO}_6$  octahedra, and the adjacent 10 La atoms was considered. The embedding potential associated with the solid-state environment was constructed from a finite array of point charges fitted to reproduce the crystal Madelung field in the cluster region [4]. We used crystal structure data as reported in Ref. 5 to construct the cluster and the embedding potential.

Effective core potentials (ECP's) and triple-zeta valence basis sets [3] were applied for the Ni ions [6]. All electron triple-zeta functions [7] were used for the oxygens of the central  $\text{NiO}_6$  octahedron whereas farther oxygens were described with minimal atomic-natural-orbital (ANO) basis sets [8]. ECP's and valence basis functions of double-zeta quality were employed for the  $\text{La}^{3+}$  species [9]. We also applied two Ni  $f$  polarization functions for the  $\text{Ni}^{2+}$  ions.

A restricted Hartree-Fock solution was first obtained for the embedded cluster. In the subsequent CASSCF calculation, a minimal active space of 5 Ni  $3d$  orbitals and 8 Ni  $3d$  electrons was considered. To make the computationally demanding MRCI calculations feasible and the analysis of the multiplet structure at the central Ni site transparent, the NN  $\text{Ni}^{2+}$  ions were “frozen” in the artificial low-spin  $t_{2g}^6 d_{3z^2-r^2}^2$  configuration, where for tetragonal distortion of the  $\text{NiO}_6$  octahedron the  $d_{3z^2-r^2}$  level is the lowest in energy within the  $e_g$  subshell, such an approach was found to be also effective in cuprates [10]. Configurations corresponding to single and double excitations involving the central-octahedron O  $2p$  and Ni  $3d$  electrons were considered in the MRCI calculations, also referred to as MR-CISD. The MOLPRO quantum chemistry package was employed for all computations [11].

The multiplet structure of the  $\text{Ni}^{2+}$  ion as obtained from MRCI calculations is compared to experimental values in Table I. Note that due to lifetime and experimental broadening nearly degenerate excitations cannot be resolved. Those MRCI relative energies are also provided

as white bars in Fig. 1(c) in the main part of the article.

### Nearest-neighbor magnetic coupling

NN magnetic coupling constants were obtained by calculations on an embedded cluster that includes two tetragonally elongated  $\text{NiO}_6$  octahedra as magnetically active units. In order to accurately describe the charge distribution in the immediate neighborhood, the 6 adjacent in-plane Ni sites and the closest 16 La ions were also incorporated in the actual cluster.

We used all-electron triple-zeta basis sets of Douglas-Kroll type for the two magnetically active Ni ions [12], all electron basis sets of quintuple-zeta quality with polarization functions for the bridging O ligand, and triple-zeta basis functions for the other “central” O’s [7]. We further employed two  $f$  polarization functions at each of the two central Ni sites [12]. As for the adjacent in-plane  $\text{Ni}^{2+}$  ions, modeled as closed-shell  $\text{Zn}^{2+}$  species, all-electron double-zeta basis sets of Douglas-Kroll type were used [12]. The La NN’s were described by ECP’s supplemented with one single  $s$  and one single  $p$  function [9, 13].

For the two reference  $\text{NiO}_6$  octahedra, the finite set of Slater determinants was defined in the CASSCF treatment in terms of 4 electrons and 4 Ni  $e_g$  orbitals. The self-consistent-field optimization was carried out for an average of the lowest singlet, triplet, and quintet states associated with this manifold. On top of the CASSCF reference, we constructed truncated MR-CISD wave functions using the difference-dedicated configuration-interaction

TABLE I. MRCI multiplet structure of the  $\text{Ni}^{2+} 3d^8$  ion in  $\text{La}_2\text{NiO}_4$ . Notations corresponding to  $D_{4h}$  point-group symmetry are used to label the various states. The leading configurations are also provided; for brevity, notations as in  $O_h$  symmetry are used for the  $3d$  orbitals. Energies relative to the  $^3B_{1g}$  ground state are given. Experimental errors correspond to 95% confidence intervals.

| $3d^8$ splittings                               | MRCI (eV) | Experimental (eV) |
|-------------------------------------------------|-----------|-------------------|
| $^3B_{1g}$ ( $t_{2g}^6 e_g^2$ )                 | 0.00      | 0.00 (1)          |
| $^3E_g$ ( $t_{2g}^5 e_g^3$ )                    | 0.86      | 1.06 (1)          |
| $^3B_{2g}$ ( $t_{2g}^5 e_g^3$ )                 | 1.56      | 1.61 (1)          |
| $^1A_{1g}$ ( $t_{2g}^6 e_g^2$ )                 | 1.56      | 1.61 (1)          |
| $^3A_{2g}$ ( $t_{2g}^5 e_g^3, t_{2g}^4 e_g^4$ ) | 1.57      | 1.61 (1)          |
| $^3E_g$ ( $t_{2g}^5 e_g^3, t_{2g}^4 e_g^4$ )    | 2.14      | 2.29 (1)          |
| $^1B_{1g}$ ( $t_{2g}^6 e_g^2$ )                 | 2.19      | 2.29 (1)          |
| $^1E_g$ ( $t_{2g}^5 e_g^3$ )                    | 2.93      | 2.93 (2)          |
| $^1B_{2g}$ ( $t_{2g}^5 e_g^3$ )                 | 3.27      | 3.35 (2)          |
| $^3A_{2g}$ ( $t_{2g}^4 e_g^4, t_{2g}^5 e_g^3$ ) | 3.47      | 3.35 (2)          |
| $^1A_{2g}$ ( $t_{2g}^5 e_g^3$ )                 | 3.66      | 3.80 (3)          |
| $^1A_{1g}$ ( $t_{2g}^6 e_g^2, t_{2g}^4 e_g^4$ ) | 3.98      | 3.80 (3)          |

(DDCI) methodology [14, 15], with all double excitations from the inactive orbital space to the virtual set of orbitals excluded. Only the Ni  $3d$  and in-plane O  $2p$  orbitals within the central two-octahedra unit were correlated in DDCI. For the DDCI calculations, we used the recently added implementation in MOLPRO [11].

### Atomic calculations

The *ab initio* quantum chemistry calculation confirms the atomic  $3d^8$  Ni configuration in  $\text{La}_2\text{NiO}_4$ , justifying the use of atomic calculations to simulate the intensity of the RIXS spectra. The approach used here is described in detail in the Supplemental Material of Ref. 16. The RIXS process at the Ni  $L$ -edge correspond to the excitation of the ground state  $2p$  level ( $2p^6 3d^8$ ) into an intermediate state ( $2p^5 3d^9$ ) that decays into the final state ( $2p^6 3d^{8*}$ ), in which  $*$  corresponds to an excited  $3d$  state. A combination of Cowan’s and Theo Thole’s codes is used to calculate the dipole transition matrices between initial, intermediate and final states using atomic wave functions mixed by *ad-hoc* crystal fields [17]. RIXS spectra are then calculated using the Kramers-Heisenberg equation [18]. The crystal fields are extracted by adjusting their values to obtain the best fit between experimental and calculated RIXS spectra.

### CHARGE STRIPE ORDER IN $\text{La}_{1.66}\text{Sr}_{0.33}\text{NiO}_4$

Hole doping  $\text{La}_2\text{NiO}_4$  drives charge and spin stripe order similar to that seen in other transition metal oxides [19]. However, the precise electronic character of doped holes remain unclear. One possibility is that holes popu-

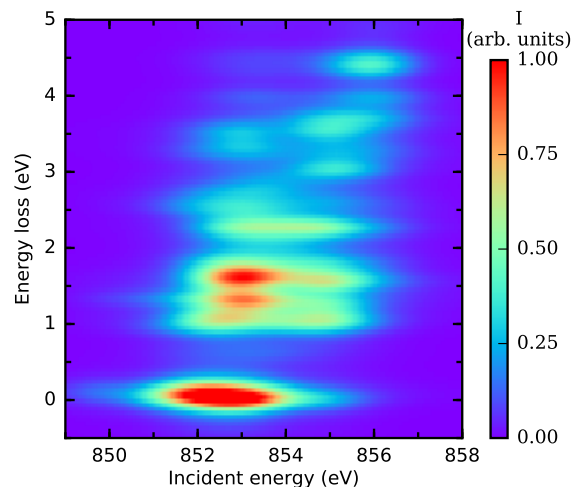

FIG. S3. Ni  $L_3$ -edge RIXS atomic calculations for a mixture of  $1/3 \times 3d^7 + 2/3 \times 3d^8$  Ni states.

late the Ni  $3d$  orbitals, leading to a mixed valence state composed of  $1/3 \times 3d^7 + 2/3 \times 3d^8$  atomic configurations. Figure S3 shows the results of Ni  $L_3$ -edge RIXS atomic calculations of such valence state using the same parameters as those described in the main text. The resulting RIXS spectra correspond to a combination of Raman-like  $3d^7$  and  $3d^8$  excitations, a very different scenario from the broad fluorescence-like feature experimentally observed (see Fig. 4 of the manuscript). The inability of this model to describe the measured RIXS spectra further implies that doping drives the Ni  $3d$  level away from an atomic character. This result is consistent with recent interpretation of NdNiO<sub>3</sub> RIXS spectra [20], and points to a dominant Ni  $3d^8\bar{L}$  state.

### LINEAR DICHROISM OF La<sub>2</sub>NiO<sub>4</sub> RIXS

Figure S4 displays the linear dichroism of the La<sub>2</sub>NiO<sub>4</sub> Ni  $L_3$ -edge RIXS spectra. Experimental data was collected using  $\theta_i = 20^\circ$  in order to isolate contributions from states oriented along  $\vec{c}$  and  $\vec{a}$  by using  $\pi$  and  $\sigma$  x-ray polarizations, respectively. The large difference observed occurs due to the distinct intermediate states along each direction: the  $\pi$  polarization leads to a  $3d^9$  intermediate state with a hole predominantly in the  $x^2 - y^2$  orbital, while with  $\sigma$  the intermediate state hole is at the  $3z^2 - r^2$  orbital. This difference does not change the excitation energies since these are independent of the intermediate state; however, the transition probabilities related to these states are different, leading to distinct

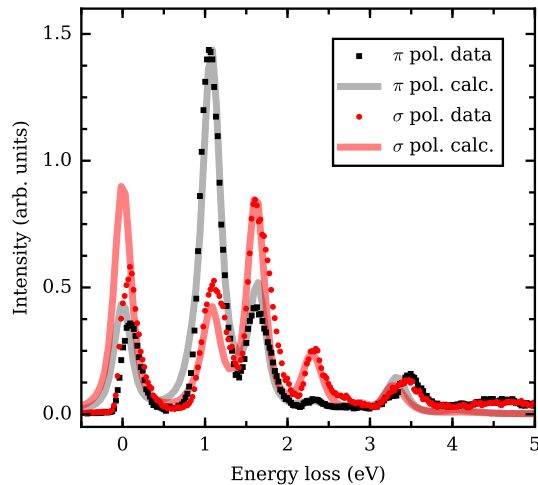

FIG. S4. Linear dichroism of the La<sub>2</sub>NiO<sub>4</sub> Ni  $L_3$ -edge RIXS spectra. Measurements were performed using  $\theta_i = 20^\circ$ , in this geometry  $\pi$  and  $\sigma$  linear polarizations primarily probe states along  $\vec{c}$  and  $\vec{a}$ , respectively. The data was normalized to the area of the orbital and charge excitations. Atomic calculations were performed in this geometry and using the parameters described in the main manuscript.

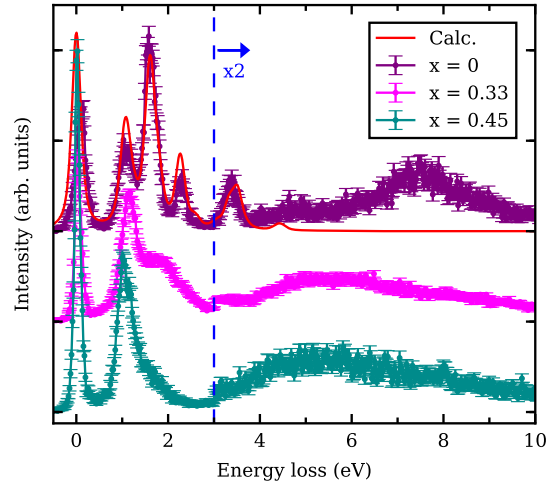

FIG. S5. Doping dependence of charge and orbital excitations in the Ni  $L_3$  of La<sub>2-x</sub>Sr<sub>x</sub>NiO<sub>4</sub>. The intensity of the spectra beyond 3 eV energy loss was multiplied by a factor of two. The data was normalized by the area of charge and orbital excitations. The spectra obtained from atomic calculations is displayed in red.

amplitudes [18]. The atomic calculations nicely capture this anisotropy, further corroborating the parameters described in the manuscript.

It is instructive to compare Fig. S4 with Fig. 4 (b)&(c) of the manuscript. The large dichroism observed in the parent compound is drastically suppressed in LSNO  $x = 0.33$ . This change supports our assessment that the doped holes strongly interact with both  $x^2 - y^2$  and  $3z^2 - r^2$  orbitals, a scenario that is distinct from cuprates, where a single band ( $x^2 - y^2$ ) interacts with the doped holes.

### DOPING DEPENDENCE OF CHARGE AND ORBITAL EXCITATIONS

Figure S5 displays the doping dependence of the RIXS spectra collected at Ni  $L_3$ -edge of LSNO. This figure allows for a direct comparison with published RIXS results for doped cuprates, including heavily doped La<sub>2-x</sub>Sr<sub>x</sub>CuO<sub>4</sub> [see for instance Fig. 1(c) of Ref. 21]. The dramatic reconstruction of excitations observed in LSNO implies that hole doping renormalizes the orbitals of nickelates more efficiently, suggesting that the doped holes acquire a larger  $3d$  character than in cuprates.

\* gfabbris@bnl.gov

† mdean@bnl.gov

[1] Kenji Nakajima, Kazuyoshi Yamada, Syoichi Hosoya, Tomoya Omata, and Yasuo Endoh, “Spin-wave excita-

- tions in two dimensional antiferromagnet of stoichiometric  $\text{La}_2\text{NiO}_4$ ,” J. Phys. Soc. Japan **62**, 4438–4448 (1993).
- [2] M. W. Haverkort, “Theory of resonant inelastic x-ray scattering by collective magnetic excitations,” Phys. Rev. Lett. **105**, 167404 (2010).
  - [3] T. Helgaker, P. Jørgensen, and J. Olsen, *Molecular Electronic-Structure Theory* (Wiley, Chichester, 2000).
  - [4] B. Roos and U. Wahlgren, MADPOT and MADFIT programs (1969).
  - [5] J. D. Jorgensen, B. Dabrowski, Shiyong Pei, D. R. Richards, and D. G. Hinks, “Structure of the interstitial oxygen defect in  $\text{La}_2\text{NiO}_{4+\delta}$ ,” Phys. Rev. B **40**, 2187–2199 (1989).
  - [6] M. Dolg, U. Wedig, H. Stoll, and H. Preuss, “Energy-adjusted *ab initio* pseudopotentials for the first row transition elements,” J. Chem. Phys. **86**, 866 (1987).
  - [7] T. H. Dunning, “Gaussian basis sets for use in correlated molecular calculations. i. the atoms boron through neon and hydrogen,” J. Chem. Phys. **90**, 1007–1023 (1989).
  - [8] Kristine Pierloot, Birgit Dumez, Per-Olof Widmark, and B. Roos, “Density matrix averaged atomic natural orbital (ano) basis sets for correlated molecular wave functions,” Theor. Chim. Acta **90**, 87–114 (1995).
  - [9] M. Dolg, H. Stoll, A. Savin, and H. Preuss, “Energy-adjusted pseudopotentials for the rare earth elements,” Theor. Chim. Acta **75**, 173–194 (1989).
  - [10] Liviu Hozoi, Liudmila Siurakshina, Peter Fulde, and Jeroen van den Brink, “*Ab Initio* determination of Cu 3d orbital energies in layered copper oxides,” Sci. Rep. **1**, 65 (2011).
  - [11] H.-J. Werner, P. J. Knowles, G. Knizia, F. R. Manby, and M. Schütz, MOLPRO 2012, see <http://www.molpro.net>.
  - [12] Nikolai B. Balabanov and Kirk A. Peterson, “Systematically convergent basis sets for transition metals. i. all-electron correlation consistent basis sets for the 3d elements sc-zn,” J. Chem. Phys. **123**, 064107 (2005).
  - [13] M. Dolg, H. Stoll, and H. Preuss, “A combination of quasirelativistic pseudopotential and ligand field calculations for lanthanoid compounds,” Theor. Chim. Acta **85**, 441–450 (1993).
  - [14] Josefa Miralles, Jean-Pierre Daudey, and Rosa Caballol, “Variational calculation of small energy differences. The singlet-triplet gap in  $[\text{Cu}_2\text{Cl}_6]^2$ ,” Chem. Phys. Lett. **198**, 555 – 562 (1992).
  - [15] Josefa Miralles, Oscar Castell, Rosa Caballol, and Jean-Paul Malrieu, “Specific CI calculation of energy differences: Transition energies and bond energies,” Chem. Phys. **172**, 33 – 43 (1993).
  - [16] G. Fabbris, D. Meyers, J. Okamoto, J. Pelliciari, A. S. Disa, Y. Huang, Z. Y. Chen, W. B. Wu, C. T. Chen, S. Ismail-Beigi, C. H. Ahn, F. J. Walker, D. J. Huang, T. Schmitt, and M. P. M. Dean, “Orbital engineering in nickelate heterostructures driven by anisotropic oxygen hybridization rather than orbital energy levels,” Phys. Rev. Lett. **117**, 147401 (2016).
  - [17] R. D. Cowan, *The Theory of Atomic Structure and Spectra* (University of California Press, Berkeley, 1981).
  - [18] Luuk J. P. Ament, Michel van Veenendaal, Thomas P. Devereaux, John P. Hill, and Jeroen van den Brink, “Resonant inelastic x-ray scattering studies of elementary excitations,” Rev. Mod. Phys. **83**, 705–767 (2011).
  - [19] J. M. Tranquada, D. J. Buttrey, V. Sachan, and J. E. Lorenzo, “Simultaneous ordering of holes and spins in  $\text{La}_2\text{NiO}_{4.125}$ ,” Phys. Rev. Lett. **73**, 1003–1006 (1994).
  - [20] Valentina Bisogni, Sara Catalano, Robert J Green, Marta Gibert, Raoul Scherwitzl, Yaobo Huang, Vladimir N Strocov, Pavlo Zubko, Shadi Balandeh, Jean-marc Triscone, George Sawatzky, and Thorsten Schmitt, “Ground-state oxygen holes and the metal-insulator transition in the negative charge-transfer rare-earth nickelates,” Nat. Commun. **7**, 13017 (2016).
  - [21] M. P. M. Dean, G. Dellea, R. S. Springell, F. Yakhov-Harris, K. Kummer, N. B. Brookes, X. Liu, Y.-J. Sun, J. Strle, T. Schmitt, L. Braicovich, G. Ghiringhelli, I. Bozovic, and J. P. Hill, “Persistence of magnetic excitations in  $\text{La}_{2-x}\text{Sr}_x\text{CuO}_4$  from the undoped insulator to the heavily overdoped non-superconducting metal,” Nat. Mater. **12**, 1018–1022 (2013).
